# Supplementary material for: Active particles with soft and curved walls: Equation of state, ratchets, and instabilities
Source: arXiv:1512.05697 ancillary file (2016-08-25)
Supplement: Supplementary file 1 [file SupplementaryInformation.pdf]

# Active particles on curved surfaces: Equation of state, ratchets, and instabilities Supplemental Material


Nikolai Nikola,[1] Alexandre P. Solon,[2,3] Yariv Kafri,[1] Mehran Kardar,[3] Julien Tailleur,[2] and Raphaël Voituriez[4,5]

[1] *Department of Physics, Technion, Haifa, 32000, Israel*
[2] *Université Paris Diderot, Sorbonne Paris Cité, MSC, UMR 7057 CNRS, 75205 Paris, France*
[3] *Massachusetts Institute of Technology, Department of Physics, Cambridge, Massachusetts 02139, USA*
[4] *Laboratoire de Physique Théorique de la Matière Condensée, UMR 7600 CNRS /UPMC, 4 Place Jussieu, 75255 Paris Cedex, France*
[5] *Laboratoire Jean Perrin, UMR 8237 CNRS /UPMC, 4 Place Jussieu, 75255 Paris Cedex*



(Dated: August 24, 2016)


Unless stated otherwise, references to figures and equations refer to those found in this Supplemental Material.

## I. SUPPLEMENTARY MOVIES

Movies can be downloaded here.

- **SI movie 1**: Coarsening of a pinned filament. Active particles are not represented. Parameters: $\kappa_s = 1000$, $\kappa_b = 250$, $r_0 = 0.3$, $\rho_0 = 1$, $v = 10$, $D_r = 1$, $L_y = 200$.
- **SI movie 2**: Motion of filaments of four different lengths. Parameters: $\kappa_s = 1000$, $\kappa_b = 250$, $r_0 = 0.3$, $\rho_0 = 1$, $v = 10$, $D_r = 1$, box size $50 \times 50$.

## II. DERIVATION OF THE EQUATION OF STATE FOR THE AVERAGED PRESSURE

We consider the dynamics of $N$ self-propelled particles that undergo rotational diffusion and randomly change orientation (tumble) in a memoryless process with rate $\alpha$. Between tumbles, the particles follow the Langevin equations

$$\begin{aligned} \partial_t \mathbf{r}_i &= v\hat{e}_{\theta_i} - \mu_t \nabla V + \sum_{j\neq i} \mathbf{F}(\mathbf{r}_i - \mathbf{r}_j) + \sqrt{2D_t}\eta_i(t) \\ \partial_t \theta_i &= \sqrt{2D_r}\eta_i^r(t), \end{aligned} \tag{1}$$

where $\mathbf{F}(\mathbf{r}_i - \mathbf{r}_j)$ is a short-range force exerted by particle $j$ on particle $i$, and $V(\mathbf{r})$ is the interaction potential between the wall and the active particles; it is periodic in $y$ with period $L_p$, vanishes in the bulk, and diverges as $x \to \infty$.

The corresponding many-body Langevin equation for the fluctuating density of particles with orientation $\theta$, $\hat{\psi}(\mathbf{r},\theta) = \sum_i \delta(\mathbf{r}-\mathbf{r}_i)\delta(\theta-\theta_i)$, is then given by [1, 2]

$$\begin{aligned} \partial_t \hat{\psi} &= -\nabla\cdot\left[v\hat{e}_\theta - \mu_t\nabla V + \mu_t \int \mathbf{F}(\mathbf{r}-\mathbf{r}')\hat{\rho}(\mathbf{r}')d^2\mathbf{r}' - D_t\nabla\right]\hat{\psi} \\ &\quad +\nabla\cdot\sqrt{2D_t\hat{\psi}}\eta + \partial_\theta\left(D_r\partial_\theta\hat{\psi} + \sqrt{2D_r\hat{\psi}}\eta^r\right) + \tfrac{\alpha}{2\pi}\int\hat{\psi}(\mathbf{r},\theta')d\theta' - \alpha\hat{\psi}, \end{aligned} \tag{2}$$

where $\hat{\rho} = \int_0^{2\pi}\hat{\psi}d\theta$ is the fluctuating particle density, $\eta(\mathbf{r},t)$ and $\eta^r(\mathbf{r},t)$ are $\delta$ correlated, zero-mean and unit-variance, Gaussian white noise fields. Let us show that the mean force per unit length exerted by the active fluid on the wall in the $\hat{x}$ direction,

$$\langle P_x\rangle \equiv \frac{1}{L_p}\int_0^{L_p} P_x(y)dy, \qquad \text{with} \qquad P_x(y) = \int_{x_\star}^{\infty} dx\rho\partial_x V, \tag{3}$$

obeys an equation of state. In the following, we denote the noise average by $\langle\cdot\rangle_\eta$ to distinguish it from the spatial average defined in Eq. (3). $x_\star$ is the abscissa of a point in the bulk far away from the wall and $\rho = \langle\hat{\rho}\rangle_\eta$ is the average particle density.

To find an expression for the pressure, following [2, 3] we first define the moments $\hat{m}_{xn} = \int_0^{2\pi}\cos(n\theta)\hat{\psi}d\theta$ and $\hat{m}_{yn} = \int_0^{2\pi}\sin(n\theta)\hat{\psi}d\theta$, such that $\hat{m}_{x0} = \hat{\rho}$, and work from now on in the steady-state. Integrating Eq. (2) over $\theta$ and averaging over the noise gives

$$0 = -\nabla\cdot\left[vm_{x1}\hat{x} + vm_{y1}\hat{y} - \mu_t\rho\nabla V + \mu_t\int\mathbf{F}(\mathbf{r}-\mathbf{r}')\langle\hat{\rho}(\mathbf{r}')\hat{\rho}(\mathbf{r})\rangle_\eta d^2\mathbf{r}' - D_t\nabla\rho\right] \equiv -\nabla\cdot\mathbf{J}, \tag{4}$$

where the average current density $\mathbf{J}$ is given by

$$\mathbf{J} \equiv vm_{x1}\hat{x} + vm_{y1}\hat{y} - \mu_t \rho \nabla V - D_t \nabla \rho + \mathbf{I}_1 (\mathbf{r}) \,, \tag{5}$$

where $m_{x,n} = \langle \hat{m}_{x,n} \rangle_\eta$, $m_{y,n} = \langle \hat{m}_{y,n} \rangle_\eta$, and $\mathbf{I}_1 (\mathbf{r}) = \mu_t \int \mathbf{F} (\mathbf{r} - \mathbf{r}') \left\langle \hat{\rho} (\mathbf{r}') \hat{\rho} (\mathbf{r}) \right\rangle_\eta d^2\mathbf{r}'$. As the system is periodic in $y$, the total flux of the current across a vertical line of length $L_p$ must vanish (see Fig. 2a of the main text:

$$\int_0^{L_p} dy J_x = 0 \,. \tag{6}$$

Integrating Eq. (6) over $x$ and using the definition of the current (5), one gets

$$\langle P_x \rangle = \frac{1}{L_p} \int_{x_\star}^{\infty} dx \int_0^{L_p} dy \rho \partial_x V = \frac{1}{L_p \mu_t} \int_{x_\star}^{\infty} dx \int_0^{L_p} dy \left( vm_{x1} - D_t \partial_x \rho + I_{1x} (\mathbf{r}) \right) , \tag{7}$$

where $I_{1x}$ is the x-component of $\mathbf{I}_1$. Next, multiplying Eq.(2) by $\cos\theta$, integrating over $\theta$, and averaging over the noise gives:

$$(D_r + \alpha) \, m_{x1} = -\nabla \cdot \left[ \hat{x} \frac{v(\rho + m_{x2})}{2} + \hat{y} \frac{vm_{y2}}{2} - \mu_t m_{x1} \nabla V - D_t \nabla m_{x1} + \mu_t \int \mathbf{F} (\mathbf{r} - \mathbf{r}') \left\langle \hat{\rho} (\mathbf{r}') \hat{m}_{x1} (\mathbf{r}) \right\rangle_\eta d^2\mathbf{r}' \right] . \tag{8}$$

We then define $\mathbf{I}_2 (\mathbf{r}) = \mu_t \int \mathbf{F} (\mathbf{r} - \mathbf{r}') \left\langle \rho (\mathbf{r}') \hat{m}_{x1} (\mathbf{r}) \right\rangle_\eta d^2\mathbf{r}'$ and integrate Eq. (8) over $x$ and $y$ to get

$$(D_r + \alpha) \int_{x_\star}^{\infty} dx \int_0^{L_p} dy m_{x1} = \int_0^{L_p} dy \left[ \frac{1}{2} v \rho (x_\star, y) + I_{2x} (x_\star, y) \right] . \tag{9}$$

Here, we have employed the fact that the r.h.s. of Eq. (8) is a divergence. Integrating the derivative with respect to $y$ over a period gives cancelling contributions while integrating the derivative with respect to $x$ between $x_\star$ and $\infty$ gives the r.h.s. of (9). Note that all moments and densities vanish at $x = \infty$ while only $\rho$ and the $x$ component of $\mathbf{I}_2$ are non-zero in the bulk. Plugging this into Eq. (7), we obtain

$$L_p \langle P_x \rangle = \left( \frac{v^2}{2\mu_t (D_r + \alpha)} + \frac{D_t}{\mu_t} \right) \int_0^{L_p} \rho (x_\star, y) \, dy + \frac{1}{\mu_t} \int_{x_\star}^{\infty} dx \int_0^{L_p} dy I_{1x} (x, y) + \frac{v}{\mu_t (D_r + \alpha)} \int_0^{L_p} dy I_{2x} (x_\star, y) \,. \tag{10}$$

Using translational invariance in the bulk, we have $\rho(x_\star, y) = \rho_0$, and similarly for $I_{2x}$, we obtain the simpler expression

$$\langle P_x \rangle = \left( \frac{v^2}{2\mu_t (D_r + \alpha)} + \frac{D_t}{\mu_t} \right) \rho_0 + \frac{v}{\mu_t (D_r + \alpha)} I_{2x}(x_\star, 0) + \frac{1}{L_p \mu_t} \int_{x_\star}^{\infty} dx \int_0^{L_p} dy I_{1x}(x, y). \tag{11}$$

This can be expressed as

$$\langle P_x \rangle = P_0 + P_I + P_D, \tag{12}$$

where $P_0$ is the 'ideal pressure' term (without interactions), as presented in the main text, $P_D$ is the direct contribution to the pressure from the pairwise forces, and $P_I$ is the indirect contribution, which is the result of having both interactions as well as self-propulsion (for a detailed discussion of the physics behind this term see [2]). The direct contribution can be simplified using Newton's third law and the periodicity of the system

$$\frac{1}{L_p \mu_t} \int_0^{L_p} dy \int_{x_\star}^{\infty} dx \int d^2\mathbf{r}' F_x (\mathbf{r} - \mathbf{r}') \left\langle \hat{\rho} (\mathbf{r}') \hat{\rho} (\mathbf{r}) \right\rangle_\eta = \frac{1}{L_p \mu_t} \int_0^{L_p} dy \int_{x > x_\star} dx \int_{x' < x_\star} F_x (\mathbf{r} - \mathbf{r}') \left\langle \hat{\rho} (\mathbf{r}') \hat{\rho} (\mathbf{r}) \right\rangle_\eta d^2\mathbf{r}', \tag{13}$$

which translates to describing the density of pair forces acting across a plane in the bulk, far from any walls.

Finally, we note that the proof for non-interacting particles, which is the focus of the main text, is a special case of the above derivation, taking $\mathbf{F} \equiv 0$.

## III. FROM FORCES TO CURRENTS

In this section, we look at the relation between the forces exerted by the active fluid on walls/objects and the particle currents in the system. The Langevin Eqs. (1) can be used to describe active particles in presence of an arbitrary

object described by a potential $V(\mathbf{r})$. The current of particles $\mathbf{J}(\mathbf{r})$ is given by Eq. (5). Consider $\mathbf{F}^{tot} = \int_S \rho \nabla V d^2\mathbf{r}$, the total force exerted on the wall/object in the region of space $S$. Similarly, we write $\boldsymbol{\mathcal{J}} = \int_S \mathbf{J} d^2\mathbf{r}$ the integrated current. Integrating Eq. (5) over the area of $S$, one obtains

$$\boldsymbol{\mathcal{J}} = -\mu_t \mathbf{F}^{tot} + \int_S \left[ v m_{x1} \hat{x} + v m_{y1} \hat{y} - D_t \nabla \rho + \mathbf{I}_1(\mathbf{r}) \right] d^2\mathbf{r}. \tag{14}$$

This equation is valid for any potential $V$ and any region $S$. In the following, we consider three cases (a wall, an isolated object and the entire system) where the integral on the r.h.s. of Eq. (14) can be evaluated to give a simple relation between currents and forces.

### A. Isolated object

We consider the case depicted in Fig. 1 (left) where the external potential $V$ has a finite extension in space, modeling an isolated object immersed in the bath of active particles. We choose a rectangular area of integration $S$ such that its boundaries are far enough from the object that they lie in the homogeneous disordered bulk of the system. Under these conditions, one can show that the integral on the r.h.s. of Eq. (14) vanishes. Indeed, Eq. (8) shows that $m_{x1}$ can be written as a divergence $m_{x1} = \nabla \cdot \mathbf{M}_{x1}$ such that, using Stokes theorem

$$\int_S v m_{x1} \hat{x} d^2\mathbf{r} = \int_\Gamma \mathbf{M}_{x1} \cdot \hat{n} dl, \tag{15}$$

where $\Gamma$ denotes the boundary of $S$ and $\hat{n}$ the normal to the boundary. Because $\Gamma$ is in the (homogeneous) bulk, $\mathbf{M}_{x1}$ is constant so that $\int_S v m_{x1} \mathbf{x} d^2\mathbf{r} = \mathbf{M}_{x1} \cdot \int_\Gamma \hat{n} dl = 0$. By similar reasoning, the second term also vanishes $\int_S v m_{y1} \hat{y} d^2\mathbf{r} = 0$. The term proportional to $D_t$ in Eq. (14) vanishes trivially. Finally, $\int_S \mathbf{I}_1$ also vanishes since, following Eq. (13), it is equal to the total forces exerted by particles outside $S$ on the active particles inside $S$. It thus vanishes by symmetry.

One thus find that the total force applied on the object by the active particles is proportional to the total flux of particles $\mathbf{F}^{tot} = -(1/\mu_t)\boldsymbol{\mathcal{J}}$. The self-propulsion of passive objects by an active bath can thus be linked to their capacity to create ratchet currents around them. Our result is exact when the distribution of active particles around the object has reached a steady state. For mobile objects of small mobilities, a quasistatic approximation on the distribution of active particles is valid and our result directly extends to this case. For smaller objects, our model has to be modified to explicitly allow for the motion of the object. Our results can be extended to this more complicated case as will be detailed in a future publication.

### B. Periodic wall

The same line of reasoning can be used to derive a relation between the vertical current and the total vertical force for the case considered in the main text where particles are confined by a periodic vertical wall. For this case, let us choose the surface $S$ such that it encompasses an integer number of periods of the wall, as depicted in Fig. 1 (center). The left boundary is taken in the bulk and the right boundary far inside the wall where the density vanishes.

Projecting Eq. (14) on the y-axis, we have

$$\mathcal{J}_y = -\mu_t F_y^{tot} + \int_S \left[ v m_{y1} - D_t \partial_y \rho + I_{1y}(\mathbf{r}) \right] d^2\mathbf{r}, \tag{16}$$

where $m_{y1}$ satisfies

$$\begin{aligned} m_{y1} = &-\frac{1}{D_r + \alpha} \nabla \cdot \left[ \hat{x} \frac{v m_{y2}}{2} + \hat{y} \frac{v(\rho - m_{x2})}{2} - \mu_t m_{y1} \nabla V - D_t \nabla m_{y1} + \mu_t \int \mathbf{F}\left(\mathbf{r} - \mathbf{r}'\right) \left\langle \hat{\rho}\left(\mathbf{r}'\right) \hat{m}_{y1}\left(\mathbf{r}\right) \right\rangle_\eta d^2\mathbf{r}' \right] \\ &\equiv \nabla \cdot \mathbf{M}_{y1}. \end{aligned} \tag{17}$$

Let us first consider the contribution of $\int_S v m_{y1} d^2\mathbf{r}$ to $\mathcal{J}_y$ in Eq. (16). Again, using Stokes theorem, it can be related to the flux of $\mathbf{M}_{y1}$ through the boundaries of $S$. $\mathbf{M}_{y1}$ vanishes on the right boundary. Let us now consider the contribution of the left boundary, for which we need to evaluate $\mathbf{M}_{y1} \cdot \hat{x}$ in the bulk of the system. First note that $m_{y2}$, $V$ and $m_{y1}$ vanish far away from the wall. Then, under reflection with respect to the $x$ axis, $\langle \hat{\rho}(\mathbf{r}') \hat{\psi}(\mathbf{r}, \theta) \sin\theta \rangle$ changes sign while $F_x$ does not. The correlator $\int \mathbf{F}\left(\mathbf{r} - \mathbf{r}'\right) \left\langle \hat{\rho}\left(\mathbf{r}'\right) \hat{m}_{y1}\left(\mathbf{r}\right) \right\rangle_\eta d^2\mathbf{r}'$ thus has non-zero component only

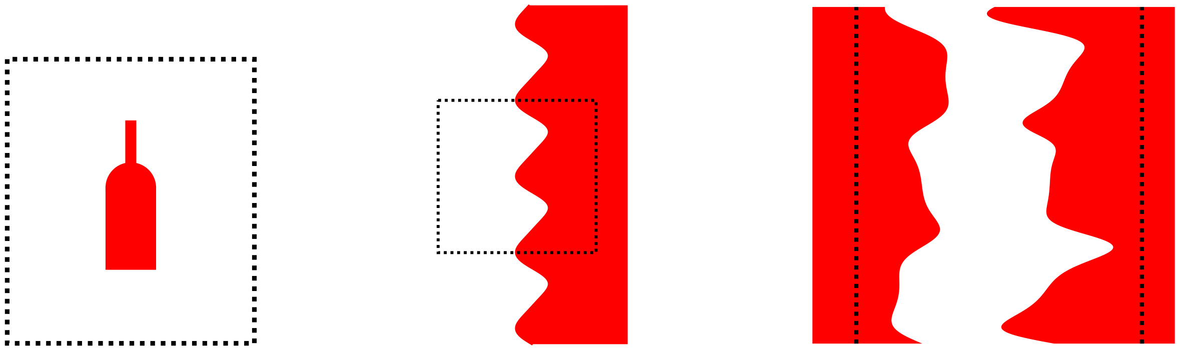

FIG. 1. The three cases considered in Sec. III. **Left:** An isolated object and the area of integration $S$ encompassing the object. **Center:** A periodic wall and the associated area of integration $S$ encompassing an integer number of periods. **Right:** Arbitrary walls confining the system in the horizontal direction.

along the $\hat{y}$ axis. All in all, $\mathbf{M}_{y1}$ thus only has contributions along the $\hat{y}$ axis and $\mathbf{M}_{y1} \cdot \hat{x} = 0$. The left boundary thus does not contribute to $\mathcal{J}_y$. Finally, the contributions of the top and bottom boundaries cancel each other because of the periodicity of the system and the choice of $S$.

Then, $\int_S D_t \partial_y \rho$ gives compensating contributions once integrated in the $\hat{y}$ direction. The last term on the r.h.s. of Eq. (16) also has vanishing contribution: It corresponds to the $y$ component of the total force exerted by particles outside $S$ onto the active particles inside $S$, i.e. the total forces exerted through the top and bottom boundaries of $S$. Because of periodicity and the third law of Newton, these two forces balance each other to yield a vanishing contribution to $\mathcal{J}_y$.

All in all, one thus obtains that $F_y^{tot} = -(1/\mu_t)\mathcal{J}_y$ where $\mathcal{J}_y$ is $\int_{x_*}^{\infty} dx J_y^{tot}$ of the main text. The shear force exerted by an active fluid on an asymmetric wall is thus proportional to the ratchet current induced by the wall.

### C. Entire system

When considering the system as the whole, the relation between the current and the total force applied on the external potential can be derived in a simpler (but equivalent way). Starting from the Langevin Eqs. (1), the current and total force can be written in terms of the particle trajectories as

$$\boldsymbol{\mathcal{J}} = \langle \sum_i \partial_t \mathbf{r}_i \rangle_\eta \qquad \mathbf{F}^{tot} = \langle \sum_i \nabla V(\mathbf{r}_i) \rangle_\eta . \tag{18}$$

Summing Eq. (1) over all particles and averaging over noise realizations, one directly gets the relation

$$\boldsymbol{\mathcal{J}} = v \langle \sum_i \hat{e}_{\theta_i} \rangle_\eta - \mu_t \mathbf{F}^{tot} + \langle \sum_i \sum_{j \neq i} \mathbf{F}(\mathbf{r}_i - \mathbf{r}_j) \rangle_\eta . \tag{19}$$

The first term on the r.h.s. of Eq. (19) vanishes because $\theta_i$ performs a random walk uncorrelated with other degrees of freedom. The last term in Eq. (19) vanishes because $\mathbf{F}(\mathbf{r}_i - \mathbf{r}_j) = -\mathbf{F}(\mathbf{r}_j - \mathbf{r}_i)$. One thus obtain the same relation as previously $\mathbf{F}^{tot} = -(1/\mu_t)\boldsymbol{\mathcal{J}}$.

For an active fluid confined in the $x$-direction by arbitrary walls with periodic boundary conditions in the y-direction (see Fig. 1, right), the flux along $\hat{x}$ vanishes so that $F_x^{tot} = 0$. The force exerted on each wall in the $x$-direction should thus be of the same magnitude.

## IV. SIMULATION DETAILS

Molecular dynamics simulations were performed employing an Euler time discretization scheme to integrate the Langevin equations (1). The time step was set at $\Delta t = 4 \times 10^{-5}$ in our simulations. At each time step, we first update the orientation and then the spatial coordinates. The run & tumble dynamics are applied by randomly choosing a time interval between tumbles from an exponential distribution with mean $\alpha^{-1}$. If the time $\tau$ for the next tumble takes place between $t_i$ and $t_{i+1}$, the interval is divided into two, a regular step takes place between $t_i$ and $\tau$, then

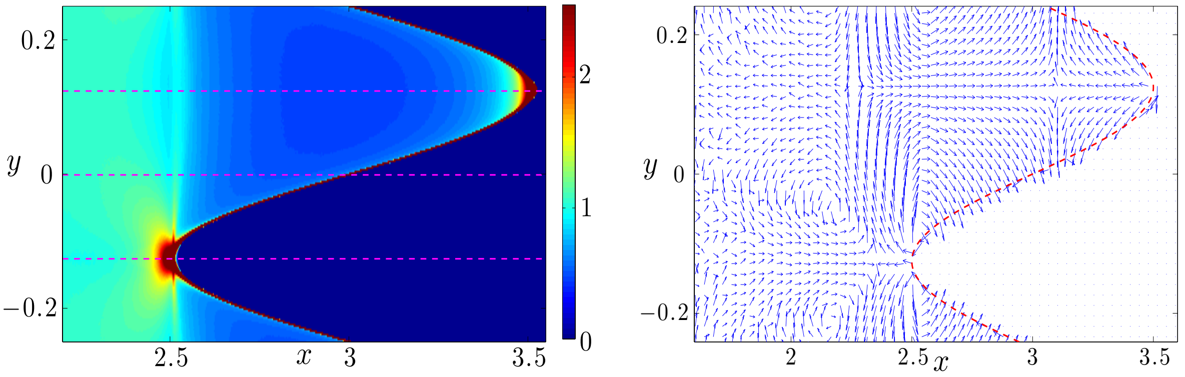


FIG. 2. Steady-state particle density (left) and current (right) of non-interacting RTPs near a hard sinusoidal wall with $\lambda = 1000$, $v = \alpha = 24$, $D_t = 0$, $L_p = 0.5$, $A = 0.5$. These parameters are identical to those of Fig.1 in the main text up to $D_r \leftrightarrow \alpha$. The dashed lines in the left figure mark the cross sections in Fig.3. The red dashed line in the right panel indicate $x_w(y)$.

a new orientation is randomly chosen from a uniform distribution, a new tumble time is chosen as before, and the particle continues its progress with its new orientation from $\tau$ to $t_{i+1}$.

Pairwise interactions derive from the Weeks-Chandler-Andersen (WCA) repulsive potential:

$$U\left(r\right) = \begin{cases} 4\varepsilon\left[\left(\frac{\sigma}{r}\right)^{12} - \left(\frac{\sigma}{r}\right)^{2}\right] + \varepsilon & \text{if } r < 2^{1/6}\sigma \\ 0 & \text{if } r > 2^{1/6}\sigma. \end{cases} \tag{20}$$

For interacting systems, the units were normalized such that $\sigma$, $\varepsilon$, and $\tau = \frac{\sigma^2}{\varepsilon\beta D_t}$, are our units of distance, energy, and time, respectively. We use $v = 24$, $\mu_t = 1$, $D_t = D_r/3$ and adjust the Peclet number $P_e = \frac{3v_0}{D_r\sigma}$ by adjusting $D_r$.

Unless stated otherwise, all simulations involved two vertical walls beginning at $x = \pm x_0$, where $x_0$ is sufficiently larger than the run length, and than $\sigma$ for interacting systems. In all simulations, we used at least $10^6$ iterations, more if needed, to ensure convergence to the steady state. The sampling for the different measurements commenced afterwards, as the system continued to evolve according to Eq. (1).

## V. SIMULATION RESULTS

### A. Run & Tumble Particles

In the main text, numerical results were shown for ABPs. Here we present similar measurements for particles with only Run & Tumble dynamics. The results are qualitatively similar to ABPs, with only limited microscopic differences (see Fig. 2). The current density presents slight differences from the ABP case, with anisotropies at larger distances from the wall, point-like confluences, and areas where the flux is inverted with respect to the one seen for ABPs. This is due to the qualitatively different behavior of ABPs and RTPs along confining walls [4]: the RTPs are able to instantaneously rotate and escape from the walls whereas the slow rotational diffusion of ABPs generates a recirculation out of the apices that takes place mostly along the walls. The pressure profile along the wall surface is, however, similar, with only slight quantitative differences (Fig.3).

These minor differences aside, as reported in the main text, the equation of state is satisfied for RTPs just as it is for ABPs. In addition, RTPs interacting with an asymmetric wall potential create tangential currents and pressures, as seen in Fig.3, in the same fashion as ABPs.

### B. Interacting Systems

Simulations of interacting systems were conducted according to the aforementioned protocol, for systems of size $L_y = 80$, vertical structured walls beginning at $x = \pm 40$ and periodic boundary conditions in the $\hat{y}$ direction. Both

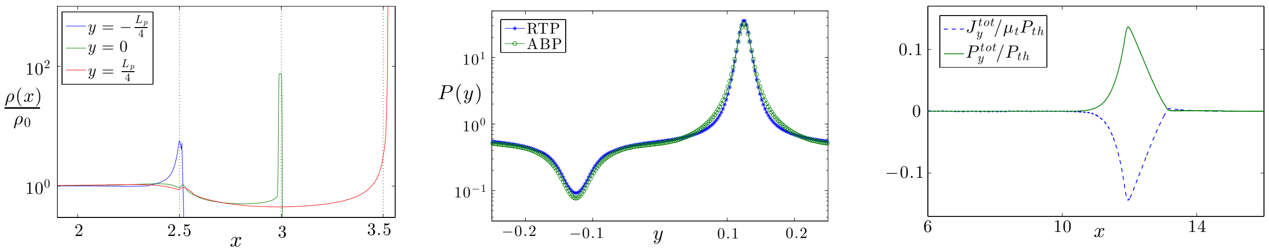


FIG. 3. **Left:** Three horizontal cross sections of the particle density in Fig.2 taken at the inner apex, the mid-point between the two apices, and the outer apex. The vertical lines mark the beginning $x_w(y)$ of the wall potential for each cross section. **Center:** The mean pressure, normal to the wall, as a function of $y$, for ABPs and RTPs. **Right:** The pressure and particle current in the $y$ direction for RTPs interacting with an asymmetrical wall potential beginning at $x_w = 10$. The potential we use is identical to that in the main text (Eq.7 and Fig3) with the same parameters.

hard sinusoidal walls and soft asymmetric walls (as in Eq.7 in the main text) were employed, with varying parameters including Peclet numbers $P_e \in [10, 90]$ , wall stiffness $\lambda \in [5, 512]$, wall period $L_p \in [0.12, 1.2]$, and bulk densities $\rho_0 \in [0.002, 0.77]$. The measured pressure in the $\hat{x}$ direction was compared to the bulk pressure predicted by the equation of state Eqs. (11).

The results, displayed in Fig. 4, confirm the validity of Eq. (11) in all regions of parameter space considered in our simulations. It also shows that $\langle P_x \rangle$ can be well estimated by measuring bulk properties, far from the walls.

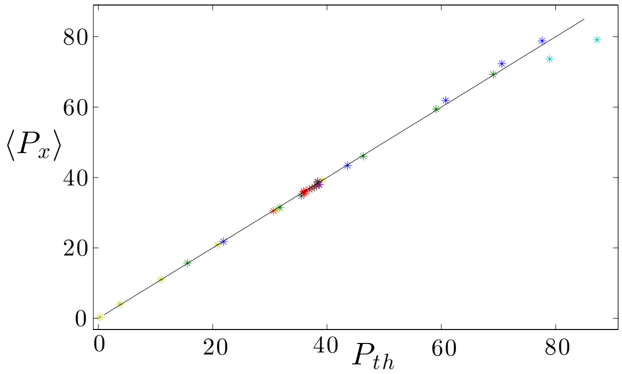


FIG. 4. The integrated pressure $\langle P_x \rangle$ for interacting systems compared with the equation of state prediction $P_{th}$ as given in Eq.(11). The data consists of 34 measurements for different parameter sets as described in the text.

## VI. INSTABILITY OF A SEMI-FLEXIBLE FILAMENT

We consider a chain of $N$ beads at positions $\mathbf{r}_i$ connected by springs with rest lengths $r_0$, spring constants $k_s$, and bending constants $k_b$. The energy of the chain is given by

$$E = \sum_{i=1}^{N} \left[ \frac{k_s}{2} \left( |\mathbf{r}_{i+1} - \mathbf{r}_i| - r_0 \right)^2 - k_b (\mathbf{t}_{i+1} \cdot \mathbf{t}_i) \right] \tag{21}$$

where $\mathbf{t}_i = (\mathbf{r}_i - \mathbf{r}_{i-1})/|\mathbf{r}_i - \mathbf{r}_{i-1}|$ is the vector tangent to the $i^{\text{th}}$ bond of the chain.

We want to study the linear stability of an initially straight chain pinned at both ends, with an initial distance $r_1$ between adjacent beads. When $r_1 > r_0$ the chain experiences a tension $T = k_s(r_1 - r_0)$. We thus consider a small bending deformation as shown in Fig. 5. Introducing the angle function $\phi(\mathbf{r}_i) \equiv \arg(\mathbf{t}_i)$, one can approximate

$$\mathbf{t}_{i+1} \cdot \mathbf{t}_i = \cos[\phi(\mathbf{r}_{i+1}) - \phi(\mathbf{r}_i)] \approx 1 - \frac{1}{2}[(\mathbf{r}_{i+1} - \mathbf{r}_i) \cdot \nabla \phi(\mathbf{r}_i)]^2 \simeq 1 - \frac{r_1^2}{2} \partial_x \phi(\mathbf{r}_i)^2 \tag{22}$$

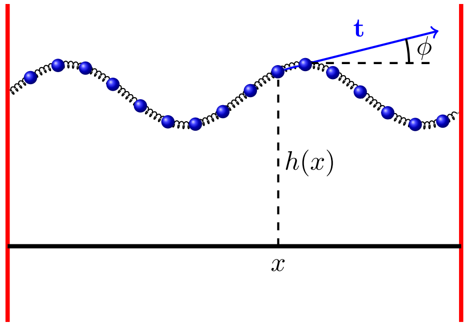


FIG. 5. Schematic representation of a fluctuation of a chain of $N$ beads pinned at its end.

where we have used that, to first order, $\mathbf{r}_{i+1} - \mathbf{r}_i \simeq r_1 \mathbf{t}_{i+1} \simeq r_1 \mathbf{u}_x$. Introducing the arc length $s(\mathbf{r}_i) = \sum_{j=0}^{i-1} |\mathbf{r}_{j+1} - \mathbf{r}_j|$, one has that $ds = |\mathbf{r}_{i+1} - \mathbf{r}_i|$ and the corresponding lateral displacement is $dx = |\mathbf{r}_{i+1} - \mathbf{r}_i| \cos[\phi(\mathbf{r}_{i+1})]$. To first order, this leads to

$$\frac{ds}{dx} \simeq \frac{|\mathbf{r}_{i+1} - \mathbf{r}_i|}{r_1}. \tag{23}$$

We now take the continuum limit $r_0 \to 0$, $N \to \infty$, while keeping the chain length $L = N r_1$, the tension $T$ and $\epsilon \equiv (r_1 - r_0)/r_1$ constant. Using the effective stretching and bending constants

$$\kappa_{s/b} \equiv \lim_{r_0 \to 0} r_1 k_{s/b} \tag{24}$$

and discarding constant terms, Eq. (21) becomes

$$E = \int_0^L \left[ \frac{\kappa_s}{2} \left( \frac{ds}{dx} - (1-\epsilon) \right)^2 + \frac{\kappa_b}{2} \left( \frac{d\phi}{dx} \right)^2 \right] dx. \tag{25}$$

To study fluctuations around a flat chain, we parametrize it by the height $h(x)$ as in Fig. 5. Using that $ds^2 = dh^2 + dx^2$ and $\frac{d\phi}{ds} \simeq h''$, we find at leading order

$$E = \int_0^L \frac{T}{2}(h')^2 + \frac{\kappa_b}{2}(h'')^2 dx. \tag{26}$$

where we used $\epsilon = T/\kappa_s$.

The numerical results shown in Fig. 2 of the main text suggest that the pressure difference on the two sides of an undulating obstacle is a function of its curvature. In Fig. 6, we show that, to first order, the pressure difference $\Delta P = P_{\max} - P_{\min}$ is simply proportional to the curvature $R$ at the tips of the sinusoidal wall: $\Delta P \equiv \gamma/R$ where $\gamma$ is an apriori unknown constant. At linear order in $h$, $1/R = \nabla^2 h$ so that, including the pressure imbalance, the dynamics of the filament in the active bath reads

$$\partial_t h(x) = [T - \gamma] \nabla^2 h - \kappa_b \nabla^4 h. \tag{27}$$

Equation (27) predicts a threshold at $\gamma = T$: At large activity $\gamma > T$, perturbations with wave number $q < q_c$ grow exponentially, with $q_c \equiv \sqrt{\frac{\gamma - T}{\kappa_b}}$, whereas if $\gamma < T$, all wavelengths are stable. To get more insight on the mechanism underlying this instability, we note that Fig. 6 shows $\gamma \propto \frac{P_0 v}{D_r}$. Here $P_0 = \rho_0 v^2/(2D_r)$ is the average pressure given by the equation of state. The coefficient $\gamma$ thus increases with the run length $v/D_r$ at fixed bulk pressure $P_0$. This results from the microscopic structure of the active fluid in the boundary layer close to the obstacle; equation (27) thus shows that immersing an elastic chain in an active bath leads to an effective reduction of its surface tension. For large activities, this effect is strong enough to induce an instability.

To estimate $q_c$, we fit the data in Fig. 6 to get the proportionnality coefficient between $\gamma$ and $\frac{P_0 v}{D_r}$, whose value is found to be $\approx 1.4$. For free filaments ($T = 0$), the parameters used in Fig.5 of the main text then give a minimal unstable filament length of $L_c = \pi\sqrt{\kappa_b/\gamma} = 1.9$ and 2.7 for $\kappa_b = 250$ and 500, respectively. These orders of magnitude are consistent with the simulation data. Note that a real active bath not only imparts a deterministic force on curved

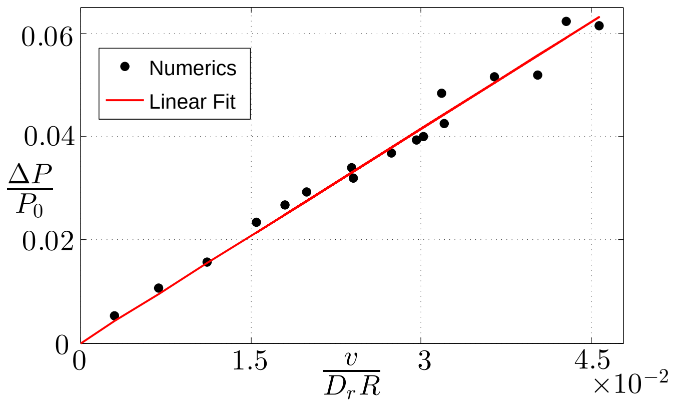


FIG. 6. Linearity of the pressure difference between the concave and convex apices of a hard sinusoidal wall ($P_{\max}$ and $P_{\min}$ in Fig.2b of the main text), normalized by $\langle P_x \rangle$ (given by the equation of state), at large radius of curvature (in units of the run lenght) $v/(D_r R)$, where $1/R = (2\pi)^2 A/L_p^2$. The red line is a linear fit of the data, forced through the origin. Numerical data were obtained from 17 ABP simulations with fixed particle parameters $v = 0.75$ and $D_r = 1$, and wall parameters in the ranges $A \in [0.0031, 0.033]$ and $L_p \in [3.6, 5.5]$, with $\lambda = 2 \times 10^4$.

regions, but also acts as a noise source. Hence, to get more accurate predictions from our linear stability analysis, all the coefficients in Eq. (27) should be replaced by effective values. In particular, even if the chain is not under tension, one expects a finite effective tension to emerge from the fluctuations of the stretching of the chain. This is why a finite treshold for the activity can be observed in the simulations reported in the main text. The linear stability analysis presented here thus gives an indication on how the microscopic constants affect the stability of the chain but we do not expect a quantitative agreement with any numerical simulations of a noisy microscopic model. Note also that Eq. (24) indicates how the microscopic constants should scale with $r_0$ in order to have a well-defined continuum limit. Using the relation between $r_1$ and $T$, one gets $\kappa_{s/b} = T + \lim_{r_0 \to 0} k_{s/b} r_0$ indicating that $k_{s/b} \propto 1/r_0$ should be used in the microscopic simulations.

[1] D. S. Dean, Journal of Physics A: Mathematical and General **29**, L613 (1996).
[2] A. P. Solon, J. Stenhammar, R. Wittkowski, M. Kardar, Y. Kafri, M. E. Cates, and J. Tailleur, Phys. Rev. Lett. **114**, 198301 (2015).
[3] A. P. Solon, Y. Fily, A. Baskaran, M. E. Cates, Y. Kafri, M. Kardar, and J. Tailleur, Nat. Phys. **11**, 673 (2015).
[4] A. Solon, M. Cates, and J. Tailleur, The European Physical Journal Special Topics **224**, 1231 (2015).
